# Supplementary material for: WGICP: Differentiable Weighted GICP-Based Lidar Odometry
Source: arXiv:2209.09777 source file (2022-10-03)
Supplement: Supplementary file 1 [file 7_supplementary.tex]

\section{Supplement}
